# Supplementary material for: Bridging the Gap between Real-world and Synthetic Images for Testing Autonomous Driving Systems
Source: arXiv:2408.13950 source file (2024-08-25)
Supplement: Supplementary file 1 [file appendix.tex]

\clearpage

For every scenario $i$, we denote the fitness function when corrector model is used as $F_{c,i}$ and the fitness function when no corrector is used as $F_{r,i}$. As both $F_{c,i}$ and $F_{r,i}$ are calculated using averaging over thousands of logs in a simulation, due to the central limit theorem, it's safe to assume they have Normal distributions. The difference between these two fitnesses is defined as $e_i = F_{c,i} - F_{r,i}$ which is also a Normal random variable. Since each scenario has its own simulation which is completely isolated from other scenarios and simulations, we can safely assume that all $e_i$s are independent and identically distributed (IID) and have Normal distribution. Let's assume that the true difference between the fitness function with and without corrector is a constant E which is unknown to us. Therefore, for each $e_i$ we have
\begin{align}
    e_i = E + n_i
\end{align}

In this formulation, $n_i$ is the flakiness effects causing the observed $e_i$ to be different from $E$. We can assume $n_i$s to be independent and identically distributed and be observations of the random variable $N$. With no loss of generality, $N$ can be considered to have zero mean. Otherwise, we can add its non-zero mean to $E$ and define new $N^\prime = N - \EX\{N\}$ to have zero mean. Additionally, we denote the variance of $N$ as $\sigma^2$.

To estimate $E$, we can use an average estimator defined by the following.

\begin{align}
    \hat{E} = \frac{1}{m} \sum_{i=1}^m e_i
\end{align}

where $m$ is the number of observations. Now, let's compute the mean value of $\hat{E}$.
\begin{align}
    \EX\{\hat{E}\} &= \frac{1}{m} \sum_{i=1}^m \EX\{e_i\}\\
    &= \frac{1}{m} m.E\\
    &= E
\end{align}
So, $\hat{E}$ is an unbiased estimator of $E$.

The variance of $\hat{E}$, denoted by $\hat{\sigma}^2$, is computed as the following.

\begin{align}
    \hat{\sigma}^2 &= \frac{1}{m^2} \sum_{i=1}^m \sigma^2\\
    &= \frac{1}{m} \sigma^2 \label{eqn:var}
\end{align}

Equation \ref{eqn:var} tells us that in order to reduce the uncertainty about the true value of $E$, we need to increase the number of observations (simulations).

Since each $e_i$ has a normal distribution, $\hat{E}$ is also a normal random variable. So, we have $\hat{E} \sim \mathcal{N}(E, \frac{\sigma^2}{m})$.

Due to Normality of $\hat{E}$, we have the following inequality \cite{??}.

\begin{align}
    p\{E - 3\hat{\sigma} \leq \hat{E} \leq E + 3\hat{\sigma}\} \approx 0.997
\end{align}

So, for each pair of corrector and ADS DNN, we have an estimator $\hat{E}$, for which we have a lowerbound and an upperbound for its $99.7\%$ confidence interval. Table \ref{tab:bounds} shows the upperbound and lowerbound for each pair.

\begin{table}[t]
    \centering
    \begin{tabular}{|l|l|l|l|}
\hline
\textbf{ADS DNN}                                          & \textbf{Translator} & \textbf{Lower Bound} & \textbf{Upper Bound} \\ \hline
\multicolumn{1}{|c|}{\multirow{3}{*}{\textbf{Chauffeur}}} & SAEVAE             & 0.48007              & 1.066571             \\ \cline{2-4} 
\multicolumn{1}{|c|}{}                                    & cycleG           & -0.28041             & 0.245871             \\ \cline{2-4} 
\multicolumn{1}{|c|}{}                                    & styleT              & 0.069131             & 0.270766             \\ \hline
\multirow{3}{*}{\textbf{Autumn}}                          & SAEVAE             & 0.684273             & 1.212431             \\ \cline{2-4} 
                                                          & cycleG           & 0.084973             & 0.475477             \\ \cline{2-4} 
                                                          & styleT              & 0.01505              & 0.304811             \\ \hline
\multirow{3}{*}{\textbf{Epoch}}                           & SAEVAE             & 0.326692             & 0.54202              \\ \cline{2-4} 
                                                          & cycleG           & 0.195825             & 0.463386             \\ \cline{2-4} 
                                                          & styleT              & 0.09629              & 0.220892             \\ \hline
\multirow{3}{*}{\textbf{Dave2}}                           & SAEVAE             & -0.01147             & 0.062059             \\ \cline{2-4} 
                                                          & cycleG           & -0.16452             & 0.195402             \\ \cline{2-4} 
                                                          & styleT              & -0.1172              & 0.036793             \\ \hline
\end{tabular}
    \caption{Lower bounds and Upper bounds for $99.7\%$ confidence intervals for estimation of E for pairs of correctors and ADS DNNs}
    \label{tab:bounds}
\end{table}

As we are interested in comparing different corrector models, let's define the aforementioned $\hat{E}$ estimators for an ADS DNN using correctors A and B as $\hat{E}_A$ and $\hat{E}_B$ respectively. We say that corrector A is better than corrector B if $\hat{E}_A > \hat{E}_B$. We define $D_{A,B} = \hat{E}_A - \hat{E}_B$. So, corrector A is better than corrector B if $D_{A,B} > 0$. A useful metric for comparing correctors A and B, considering flakiness, would be the probability of $D_{A,B}$ being positive. In other words, we are interested in finding $p\{D_{A,B} > 0\}$. Since $D_{A,B}$ is defined as the sum (subtraction) of two Normal random variables, it has a Normal distribution. So, we have

\begin{align}
    D_{A,B} \sim \mathcal{N}(\hat{\mu}_{A,B}, \hat{\sigma}_{A,B}^2)
\end{align}

where $\hat{\mu}_{A,B} = \hat{E}_A - \hat{E}_B$ and $\hat{\sigma}_{A,B}^2 = \hat{\sigma}_A^2 + \hat{\sigma}_B^2$. 
Since $D_{A,B}$ is Normal random variable, we have

\begin{align}
    p\{D_{A,B} > 0 \} &= 1 - F(0) \\
    &= \frac{1}{2} [1 - \text{erf}(- \frac{\hat{\mu}_{A,B}}{\hat{\sigma}_{A,B} \sqrt{2}})]
\end{align}

Table \ref{tab:p_d} shows the probability of SAEVAE being better than CycleGAN and Style for each ADS DNN.

\begin{table}[t]
    \centering
    \begin{tabular}{|l|l|l|l|}
\hline
\textbf{ADS DNN}                                          & \textbf{Translator A} & \textbf{Translator B} & $p\{D_{A,B} > 0\}$ \\ \hline
\multicolumn{1}{|c|}{\multirow{2}{*}{\textbf{Chauffeur}}} & SAEVAE               & cycleG             & 1          \\ \cline{2-4} 
\multicolumn{1}{|c|}{}                                    & SAEVAE               & styleT                & 1          \\ \hline
\multirow{2}{*}{\textbf{Autumn}}                          & SAEVAE               & cycleG             & 1          \\ \cline{2-4} 
                                                          & SAEVAE               & styleT                & 1          \\ \hline
\multirow{2}{*}{\textbf{Epoch}}                           & SAEVAE               & cycleG             & 0.966      \\ \cline{2-4} 
                                                          & SAEVAE               & styleT                & 1          \\ \hline
\multirow{2}{*}{\textbf{Dave2}}                           & SAEVAE               & cycleG             & 0.564      \\ \cline{2-4} 
                                                          & SAEVAE               & styleT                & 0.989      \\ \hline
\end{tabular}
    \caption{Probability of SAEVAE being better than other correctors for each ADS DNN}
    \label{tab:p_d}
\end{table}
